# Supplementary material for: Stochasticity from function -- why the Bayesian brain may need no noise
Source: arXiv:1809.08045 source file (2019-08-24)
Supplement: Supplementary file 1 [file newcommands.tex]

% renewed commands

\renewcommand{\and}{{\mathrm{and}}\xspace}

% command shorthands

% math shorthands

% new symbols

% indices with \mathrm stuff

% text in equations stuff

% code stuff

% environment stuff

% vitali osumness

 % Gap between visible & hidden units
 % Horizontal gap between neurons
\tikzstyle{neuron}=[circle,fill=black!25,minimum size=21pt,inner sep=0pt]
\tikzstyle{visible neuron}=[neuron, fill=green!50]
\tikzstyle{hidden neuron}=[neuron, fill=orange!75]
